# Supplementary material for: Plugging Self-Supervised Monocular Depth into Unsupervised Domain Adaptation for Semantic Segmentation
Source: arXiv:2110.06685 source file (2021-10-13)
Supplement: Supplementary file 1 [file supp_D4_UDA.pdf]

# Supplementary Material For
# Plugging Self-Supervised Monocular Depth into Unsupervised Domain Adaptation for Semantic Segmentation

Adriano Cardace Luca De Luigi Pierluigi Zama Ramirez Samuele Salti Luigi Di Stefano
Department of Computer Science and Engineering (DISI)
University of Bologna, Italy
{adriano.cardace2, luca.deluigi4, pierluigi.zama}@unibo.it

## 1. Additional Implementation Details

As stated in Sec. 3.1 of the main paper, we obtain depth proxy-labels by deploying a self-supervised method for solving monocular depth estimation from video sequences. Specifically, we train Monodepth2 [6] following the training protocol and hyper-parameters used in the original paper. We train it for 20 epochs using mixed mini-batch of size 6, composed of 3 real and 3 synthetic images. We resize samples at resolution 1024×512 for training and testing. It is important to train the network on both domains jointly because we want depth predictions to be *aligned* across domains. Self-supervised depth methods typically estimates depth maps up to a scale-factor. Thus, we train on both domains simultaneously to force the network to yield predictions from the two domains that share the same range and scale. When $\mathcal{D}_{\mathcal{S}}$ is synthetic, we can collect depth ground-truth labels with minimum effort. In such case, we could exploit these labels to provide an additional source of supervision to Monodepth2. SYNTHIA-SEQ provides much less images with smaller variability with respect to GTA5, but provides depth ground-truth labels. Thus, in the SYNSEQ→CS setting, we could train Monodepth2 by adding a $L_1$ loss between predictions and ground-truths of SYNTHIA-SEQ to the set of Monodepth2 losses, so as to achieve better pseudo-labels results. Nevertheless, the availability of ground-truth labels is not crucial to improve the performance of the considered UDA method. Indeed, in Tab. 1 we can observe that the use of synthetic depth ground-truth labels provides just a slight performance improvement (i.e. 1% mIoU or less).

As regards the training of semantics prediction from depth features, we follow the protocol explained in [9]. We train the depth network simultaneously on $\mathcal{D}_{\mathcal{S}}$ and $\mathcal{D}_{\mathcal{T}}$, by minimizing the mean absolute error (i.e. $L_1$ loss) between predicted depth maps and depth proxy-labels, previously generated for both domains. Then, we train the semantic network only on $\mathcal{D}_{\mathcal{S}}$, using a weighted Cross Entropy loss with weights computed as in [18]. The weights of the two networks are pre-initialized on ImageNet, and, following a common protocol [14, 18, 7], all Batch Normalization layers are frozen both at training and test time to use ImageNet statistics. Differently from [9], we deploy the more performant DeepLabV2 [1] architecture for both networks: as the framework requires to split the network into an encoder and a decoder, we consider the backbone as the encoder and the ASPP module as the decoder. Hence, the transfer function in D4 is learned by minimizing the mean squared distance (i.e. $L_2$ loss) between the semantic features extracted by the semantic network encoder and the ones hallucinated by the transfer function itself starting from the depth encoder. Finally, during DBST, the final distilled model is obtained by minimizing a standard Cross Entropy loss on $\mathcal{D}_{\mathcal{T}}$ and exploiting only the pseudo-labels, as explained in Sec. 3.2 of the main paper.

## 2. Additional Datasets Details

**Cityscapes**. The Cityscapes dataset [4] provides a large collection of video sequences of driving scenes from 50 different European cities. The dataset is composed of 150000 video-sequence images, of which 83300 are used for training. A subset of 5000 images from Cityscapes is commonly used as benchmark for semantic segmentation, as these images are annotated with high-quality pixel-level semantic labels (19 classes). This subset is split into train, validation and test with 2975, 500 and 1525 images respectively. In our experiments we train Monodepth2 [6] on the 83300 training sequences. For training D4 and DBST we use the 2975 train images (without their semantic labels) and, following the protocol adopted in recent works [14, 2, 8, 18, 17, 16, 7], we evaluate our final model on the validation split. The augmented dataset obtained during DBST starting from the 2975 images accounts for 7500 samples.

**GTA5**. The GTA5 dataset [10, 11] consists in synthetic

images captured while playing the video-game Grand Theft Auto V. It consists of 120000 video-sequence images that we use in the Monodepth2 [6] training procedure. Moreover, the dataset provides 24966 samples with fine semantic annotations (same 19 classes as Cityscapes). We train the depth network of D4 on only 3000 randomly sampled images among the 24966 to keep the training balanced with the 2975 images of Cityscapes. Finally, we train the semantic and transfer network of D4 on the whole 24966 synthetic images.

**SYNTHIA VIDEO SEQUENCES**. The SYNTHIA dataset [12] is composed of images generated by rendering a virtual city created with the Unity development platform. Since our method requires video sequences to train Monodepth2 [6], we use the split SYNTHIA VIDEO SEQUENCES, selecting sub-sequences *Spring*, *Summer*, *Fall*, *Winter*, *Dawn* and *Fog*. We collect thus a total of 26948 images, paired with fine-grained semantic labels (12 classes in common with Cityscapes). In particular, we train on *sky*, *building*, *road*, *sidewalk*, *fence*, *vegetation*, *pole*, *car*, *traffic sign*, *person*, *bicycle*, *traffic light*. It is worth noticing that to make the Cityscapes dataset consistent with SYNTHIA VIDEO SEQUENCES, it is necessary to map the Cityscapes class *rider* into *bicycle* and collapse *bus* and *truck* into *car*. We use only 3000 randomly sampled images to train the depth, semantic and transfer network of D4, as well as for the training of the other considered methods which were retrained by us (* in Tab. 2 of the main paper) due to the authors not providing their results on SYNTHIA VIDEO SEQUENCES.

## 3. Semantics From Depth

In this section, we evaluate alternative ways to predict semantics in the target domain by exploiting also the depth cues available once depth proxy-labels have been computed as discussed in sec 3.1 (*Semantics from depth*) of the main paper. This study motivates our choice to rely on the mechanism of transferring features across tasks and domains [9], with the improvements and modifications discussed in Sec. 4.1 of the main paper and Sec. 1 of this supplementary document. As we have semantic labels only for the source domain $\mathcal{D}_\mathcal{S}$, all approaches are trained only on $\mathcal{D}_\mathcal{S}$, and their ability to generalize is assessed on the target domain $\mathcal{D}_\mathcal{T}$.

We investigate two possible alternatives, namely:

- a semantic segmentation network that processes RGB-D images, where the proxy depth of each image is stacked as an additional channel
- a semantic segmentation network that processes directly proxy depths, without using RGB information.

We realize both options by training the popular DeepLabV2 [1] architecture to perform semantic segmentation on $\mathcal{D}_\mathcal{S}$, initializing the network with ImageNet [5] pre-trained weights. Moreover, in the first case, we add a convolutional layer at the beginning of the architecture, to reduce the input RGBD channels from 4 to 3, while in the second case we obtain 3-channels input images by stacking three times the proxy depth map. In the following, we will call DeepLabV2-RGBD the first network and DeepLabV2-Depth the second one. We also consider as baseline the performance of DeepLabV2 trained only on RGB images, referred to as DeepLabV2-RGB.

| Method | mIoU |
|---|---|
| AdaptSegNet* [14] | 49.5 |
| D4-AdaptSegNet + DBST (w/o synthetic GT) | 55.9 |
| D4-AdaptSegNet + DBST (w/ synthetic GT) | 56.9 |
| MaxSquare* [2] | 51.2 |
| D4-MaxSquare + DBST (w/o synthetic GT) | 56.5 |
| D4-MaxSquare + DBST (w/ synthetic GT) | 57.4 |
| MRNET* [18] | 54.5 |
| D4-MRNET + DBST (w/o synthetic GT) | 55.9 |
| D4-MRNET + DBST (w/ synthetic GT) | 56.3 |

Table 1. Results on the SYNSEQ→CS benchmark with or without synthetic ground-truths. * denotes method retrained by us.

In Tab. 2 we report mIoU results obtained on Cityscapes (i.e. our target domain) by DeepLabV2-RGB, DeepLabV2-RGBD, DeepLabV2-Depth, and our method. We observe that the RGBD and the Depth versions yield slightly better results compared to the RGB baseline. Interestingly, DeepLabV2-Depth provides better results than DeepLabV2-RGB and DeepLabV2-RGBD, which supports our intuition about semantic cues extracted from depth alone being more effectively transferable across different domains due to their reliance on geometry rather than appearance. Yet, the ability to overcome the domain shift by DeepLabV2-RGBD and DeepLabV2-Depth is limited, as performance is low for both variants. On the contrary, by tackling the problem with the method proposed in the main paper, we can improve the baseline by 8.6% in terms of mIoU.

Moreover, we evaluate DeepLabV2-RGBD and DeepLabV2-Depth also in combination with an UDA method, as proposed in Sec. 3.1 (*Combine with UDA*) of the main paper. In the last three rows of Tab. 2, we report mIoU results obtained by such combinations (row 5 and 6), compared to our proposal (last row), while considering one of the best performing UDA methods, namely LTIR [7]. As intuitively expected, we observe that a better depth-based semantic model leads to a better combination with the selected UDA method, motivating once again the need for an approach robust to domain-shift in order to infer semantics from depth cues in UDA settings.

Rather than relying on self-supervised depth on both do-

| Method | mIoU |
|---|---|
| DeepLabV2 RGB | 34.5 |
| DeepLabV2-RGBD | 35.5 |
| DeepLabV2-Depth | 36.5 |
| Semantics from depth (sec 3.1) | **43.1** |
| DeepLabV2-RGBD $\bigoplus$ LTIR [7] | 47.7 |
| DeepLabV2-Depth $\bigoplus$ LTIR [7] | 49.3 |
| D4-LTIR (*i.e.* Semantics from depth $\bigoplus$ LTIR) | **51.1** |

Table 2. Comparison between alternative methods to infer semantics with the aid of depth cues. DeepLabV2-RGB, DeepLabV2-RGBD and DeepLabV2-Depth stand for DeepLabV2 [1] trained on $\mathcal{D}_\mathcal{S}$, using respectively RGB images, RGBD images or depth proxy-labels as input, while "Semantics from depth" is the approach described in the subsection with the same name of sec 3.1 in the main paper. The symbol $\bigoplus$ represents the merge operation described in subsection *Combine with UDA* of Sec. 3.1 of the main paper. Results are reported in terms of mIoU on the Cityscapes dataset.

mains as done for the previous cases, one may try to use just the depth provided by synthetic source dataset. To the best of our knowledge, only two works [15, 3] proposed to exploit depth in a UDA context for outdoor scenes segmentation. We compare here our D4 module with [15], the only publicly available framework, to show that the additional information for the target domain is a key component for Domain Adaptation. We retrained [15] with the same hyper-parameters, and changed only the training split (i.e. SYNTHIA-SEQ instead of SYTNHIA-RAND-CITYSCAPES). As Tab 3 shows, D4 surpasses by a large margin (3.6%) [15], suggesting that self-supervised information for the target domain can be used to boost performance in Domain Adaptation.

| Method | mIoU |
|---|---|
| DADA [15] | 42.3 |
| D4 (ours) | 45.9 |

Table 3. Comparison between depth-based frameworks.

## 4. DBST vs DACS [13]

In Tab. 4 we compare our DBST with the method presented in DACS [13], as they share some similarities. In particular, both approaches generate training samples by *copying* portions of images onto other images. However, they differ in three main aspects:

- [13] copies portions of images from $\mathcal{D}_\mathcal{S}$ onto images from $\mathcal{D}_\mathcal{T}$, while in our DBST we use exclusively images from $\mathcal{D}_\mathcal{T}$.
- In our proposal, we copy only image patches whose semantic predictions belong to a predefined set of classes that we deem as more amenable to be moved across images, like, e.g., *person*, *car* and *pole*; conversely, in [13] no semantic filter is applied to select the patches that will be copied across the images.
- Unlike [13], we exploit depth information to plausibly stack objects in the generated sample.

| Method | mIoU |
|---|---|
| D4-LTIR [7] | 51.1 |
| D4-LTIR [7] + DACS [13] | 52.7 |
| D4-LTIR [7] + DBST | **54.1** |

Table 4. Comparison between the approach proposed in [13] (DACS) and our DBST, when applied to our D4 combined with [7]. Results are reported in terms of mIoU in the GTA5→CS benchmark.

| Method | mIoU |
|---|---|
| AdaptSegNet (w/o video) [14] | 42.4 |
| AdaptSegNet (w/ video) | 41.9 |

Table 5. AdaptSegNet [14] trained with or without additional unlabeled target images

In addition to these points, in our DBST we further exploit depth information to guide the selection of the patches to be copied by excluding areas of the scene that are too far away from the camera, where semantic predictions are less likely accurate. In Tab. 4 we report results in the GTA5→CS benchmark when applying DBST or [13] to D4 combined with [7]: our DBST outperforms the strategy proposed in [13], though the latter can also yield a notable performance improvement.

## 5. Adding videos to UDA methods

In this section, we empirically demonstrate that using additional raw information is not directly useful for the UDA setting in semantic segmentation. To this purpose, we adopt [14], which makes use of adversarial training and it can be considered as the main building block of many UDA methods proposed in the literature. Moreover, adversarial training is a plausible strategy to exploit additional unlabeled images for the target domain. Driven by this reasoning, we retrained [14] in the GTA5→CS benchmark using the whole training split available in Cityscapes (i.e. 83300 images with temporal consistency). The result reported in Tab. 5 suggests that simply collecting more data is not enough to boost semantic semantic segmentation in a UDA setting, and more advanced techniques as the one proposed in this work are necessary to extrapolate useful data.

## 6. Qualitative Results

In Fig. 1, 2, 3, 4, 5, 6 we report several qualitative results of our D4 proposal combined with the different UDA methods reported in Tab. 1 and Tab. 2 of the main paper. In every case, we observe an overall improvement in the quality of the predictions. In particular, thanks to the additional information provided by depth maps, the errors in large objects with regular shapes are partially removed (see first and second column of Fig. 1). Moreover, with the proposed merging algorithm (Sec 3.1) and with the DBST algorithm detailed in Sec. 3.2, we also preserve the good performance of the selected UDA method for certain classes. For instance, all the predictions concerning classes such as *pole* and *traffic sign* are always maintained or even improved (see second row of Fig. 2).

## 7. DBST - Qualitative Results

In Fig. 7 and 8 we show some training samples obtained with our DBST algorithm. As explained in Sec. 3.2 of the main paper, we use multiple images from $\mathcal{D}_\mathcal{T}$ as source, alongside with the corresponding depth maps and predictions (referred to as pseudo-labels), to synthesize new training pairs. We can notice how the newly generated samples contain a lot of patterns that would not be present in the original images, enabling a more effective Self-Training procedure. We also point out how, thanks to the use of depth maps, the generated pairs look realistic. For example, in the third row of Fig. 7, the rider on the left side of the image is pasted in front of the pole since it appears closer in the depth maps of the two images.

## 8. Depth Proxy-Labels

Fig. 9, 10, 11 report depth proxy-labels obtained in the first step of our pipeline by the self-supervised approach proposed in Monodepth2 [6]. We note how the produced depth maps are smooth and accurate on the static parts of the scene (such as road and buildings), while they tend to be noisy on moving objects (like cars and pedestrians). Despite these imperfections, depth proxy-labels produced by [6] provide a solid base of geometric clues for objects with large and regular shapes, which are extensively exploited in our proposal.

## References


[1] Liang-Chieh Chen, George Papandreou, Iasonas Kokkinos, Kevin Murphy, and Alan L. Yuille. Deeplab: Semantic image segmentation with deep convolutional nets, atrous convolution, and fully connected crfs. *IEEE Transactions on Pattern Analysis and Machine Intelligence*, 40(4):834–848, Apr 2018. 1, 2, 3

[2] Minghao Chen, Hongyang Xue, and Deng Cai. Domain adaptation for semantic segmentation with maximum squares loss. *2019 IEEE/CVF International Conference on Computer Vision (ICCV)*, Oct 2019. 1, 2, 6, 8

[3] Yuhua Chen, Wen Li, Xiaoran Chen, and Luc Van Gool. Learning semantic segmentation from synthetic data: A geometrically guided input-output adaptation approach. *2019 IEEE/CVF Conference on Computer Vision and Pattern Recognition (CVPR)*, Jun 2019. 3

[4] Marius Cordts, Mohamed Omran, Sebastian Ramos, Timo Rehfeld, Markus Enzweiler, Rodrigo Benenson, Uwe Franke, Stefan Roth, and Bernt Schiele. The cityscapes dataset for semantic urban scene understanding. In *The IEEE Conference on Computer Vision and Pattern Recognition (CVPR)*, June 2016. 1

[5] J. Deng, W. Dong, R. Socher, L. Li, Kai Li, and Li Fei-Fei. Imagenet: A large-scale hierarchical image database. In *2009 IEEE Conference on Computer Vision and Pattern Recognition*, pages 248–255, 2009. 2

[6] Clement Godard, Oisin Mac Aodha, Michael Firman, and Gabriel Brostow. Digging into self-supervised monocular depth estimation. *2019 IEEE/CVF International Conference on Computer Vision (ICCV)*, Oct 2019. 1, 2, 4, 11

[7] Myeongjin Kim and Hyeran Byun. Learning texture invariant representation for domain adaptation of semantic segmentation. *2020 IEEE/CVF Conference on Computer Vision and Pattern Recognition (CVPR)*, Jun 2020. 1, 2, 3, 7

[8] Yunsheng Li, Lu Yuan, and Nuno Vasconcelos. Bidirectional learning for domain adaptation of semantic segmentation. *2019 IEEE/CVF Conference on Computer Vision and Pattern Recognition (CVPR)*, Jun 2019. 1, 7

[9] Pierluigi Zama Ramirez, Alessio Tonioni, Samuele Salti, and Luigi Di Stefano. Learning across tasks and domains. *2019 IEEE/CVF International Conference on Computer Vision (ICCV)*, Oct 2019. 1, 2

[10] Stephan R. Richter, Zeeshan Hayder, and Vladlen Koltun. Playing for benchmarks. In *IEEE International Conference on Computer Vision, ICCV 2017, Venice, Italy, October 22-29, 2017*, pages 2232–2241, 2017. 1

[11] Stephan R. Richter, Vibhav Vineet, Stefan Roth, and Vladlen Koltun. Playing for data: Ground truth from computer games. *Lecture Notes in Computer Science*, page 102–118, 2016. 1

[12] German Ros, Laura Sellart, Joanna Materzynska, David Vazquez, and Antonio M. Lopez. The synthia dataset: A large collection of synthetic images for semantic segmentation of urban scenes. In *The IEEE Conference on Computer Vision and Pattern Recognition (CVPR)*, June 2016. 2

[13] Wilhelm Tranheden, Viktor Olsson, Juliano Pinto, and Lennart Svensson. Dacs: Domain adaptation via cross-domain mixed sampling. In *Proceedings of the IEEE/CVF Winter Conference on Applications of Computer Vision (WACV)*, pages 1379–1389, January 2021. 3

[14] Yi-Hsuan Tsai, Wei-Chih Hung, Samuel Schulter, Kihyuk Sohn, Ming-Hsuan Yang, and Manmohan Chandraker. Learning to adapt structured output space for semantic segmentation. *2018 IEEE/CVF Conference on Computer Vision and Pattern Recognition*, Jun 2018. 1, 2, 3, 6, 8

[15] Tuan-Hung Vu, Himalaya Jain, Maxime Bucher, Matthieu Cord, and Patrick Perez Perez. Dada: Depth-aware domain

adaptation in semantic segmentation. *2019 IEEE/CVF International Conference on Computer Vision (ICCV)*, Oct 2019. 3

[16] Haoran Wang, Tong Shen, Wei Zhang, Lingyu Duan, and Tao Mei. Classes matter: A fine-grained adversarial approach to cross-domain semantic segmentation. In *The European Conference on Computer Vision (ECCV)*, August 2020. 1

[17] Zhonghao Wang, Mo Yu, Yunchao Wei, Rogerio Feris, Jinjun Xiong, Wen-mei Hwu, Thomas S. Huang, and Honghui Shi. Differential treatment for stuff and things: A simple unsupervised domain adaptation method for semantic segmentation. *2020 IEEE/CVF Conference on Computer Vision and Pattern Recognition (CVPR)*, Jun 2020. 1

[18] Zhedong Zheng and Yi Yang. Unsupervised scene adaptation with memory regularization in vivo. *Proceedings of the Twenty-Ninth International Joint Conference on Artificial Intelligence*, Jul 2020. 1, 2

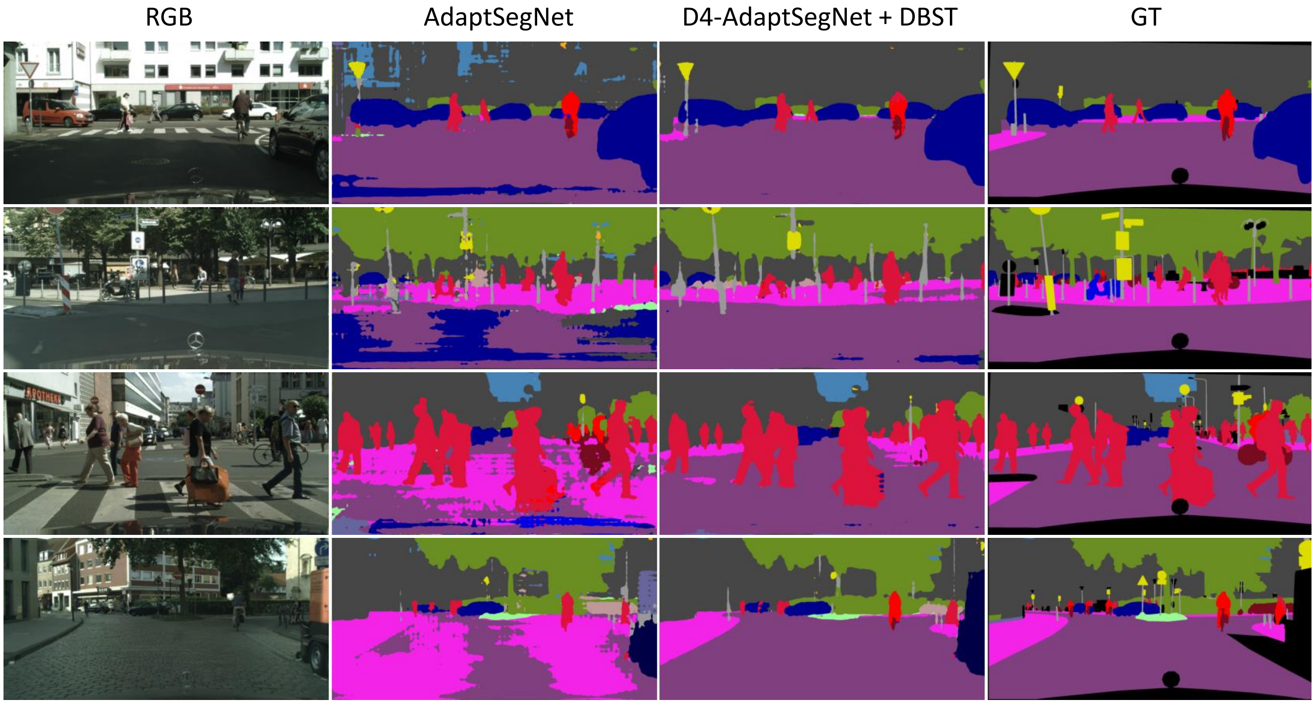


Figure 1. Qualitative results in the GTA5→CS benchmark. From left to right: RGB, prediction from Adaptsegnet [14], prediction from D4-AdaptSegNet + DBST (our proposal), Ground-Truth.

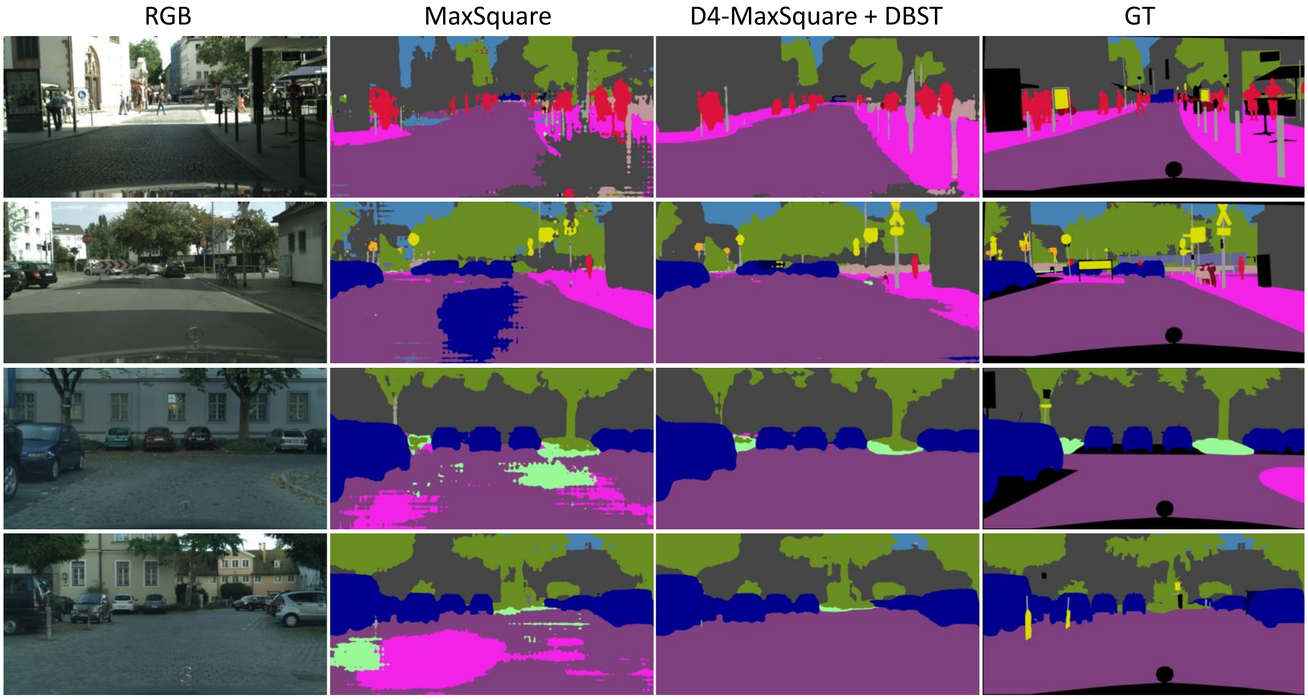


Figure 2. Qualitative results in the GTA5→CS benchmark. From left to right: RGB, prediction from MaxSquare [2], prediction from D4-MaxSquare + DBST (our proposal), Ground-Truth.

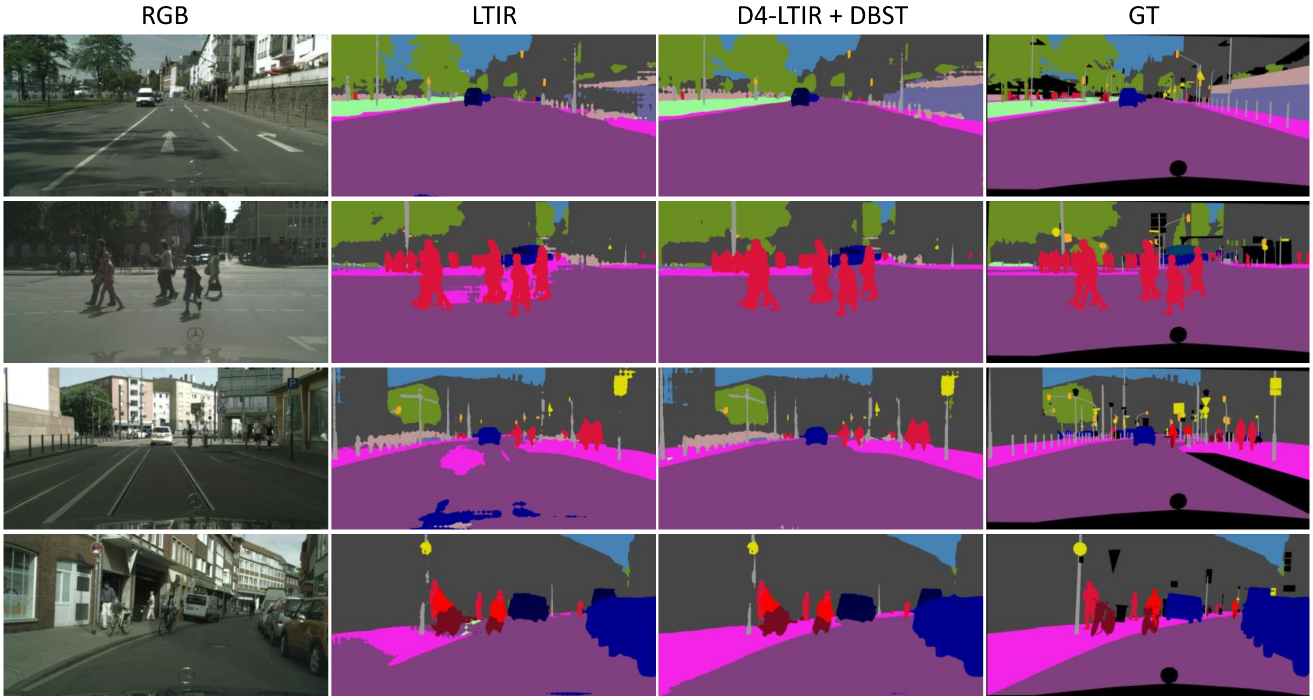


Figure 3. Qualitative results in the GTA5→CS benchmark. From left to right: RGB, prediction from LTIR [7], prediction from D4-LTIR + DBST (our proposal), Ground-Truth.

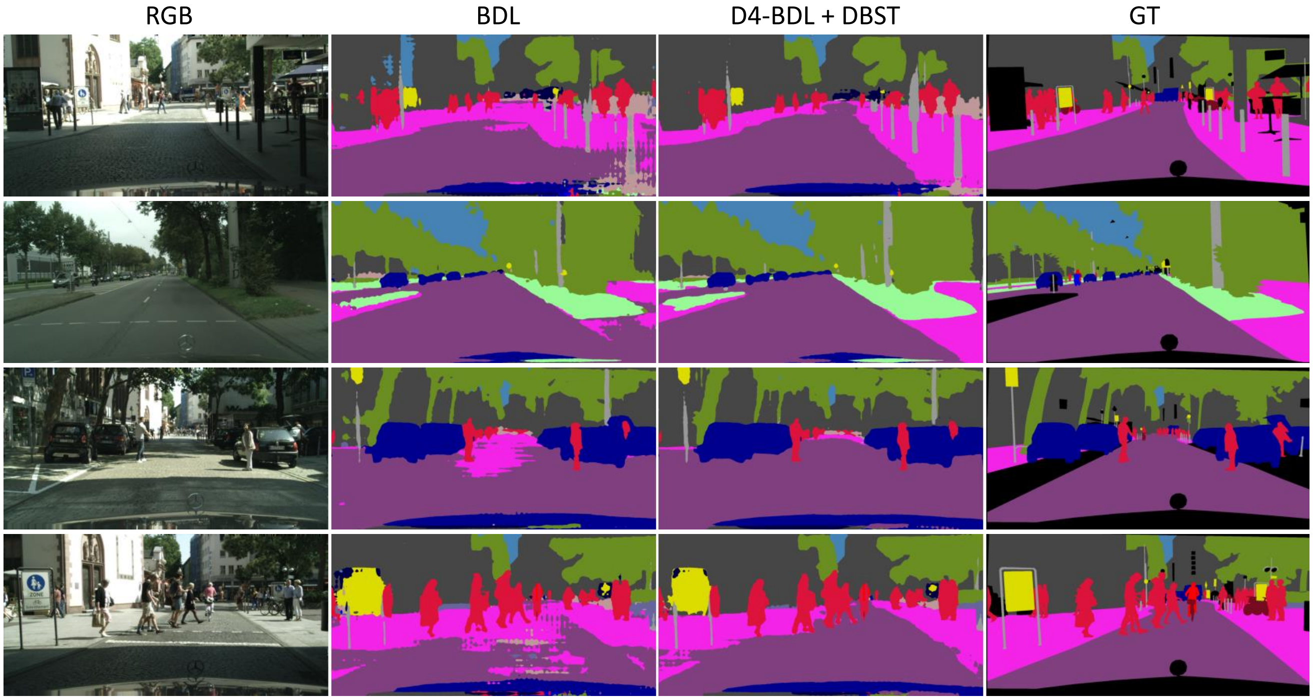


Figure 4. Qualitative results in the GTA5→CS benchmark. From left to right: RGB, prediction from BDL [8], prediction from D4-BDL + DBST (our proposal), Ground-Truth.

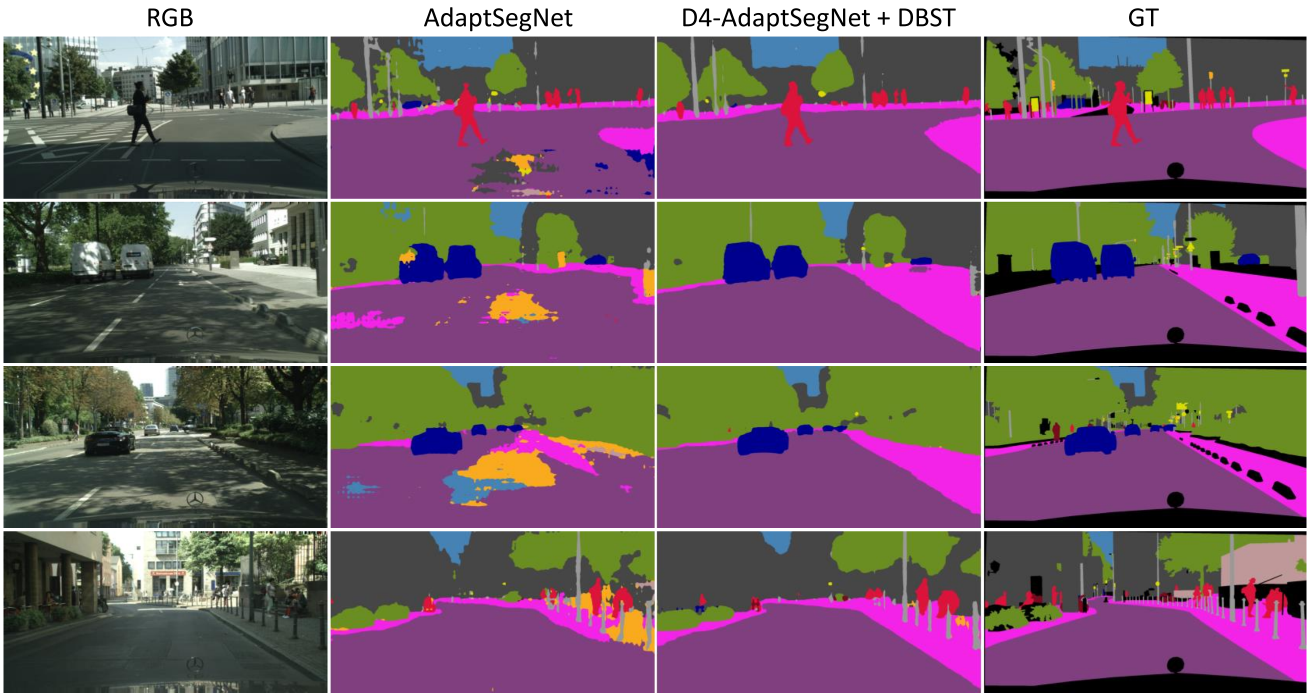


Figure 5. Qualitative results in the SYNSEQ→CS benchmark. From left to right: RGB, prediction from AdaptSegNet [14], prediction from D4-AdaptSegNet + DBST (our proposal), Ground-Truth.

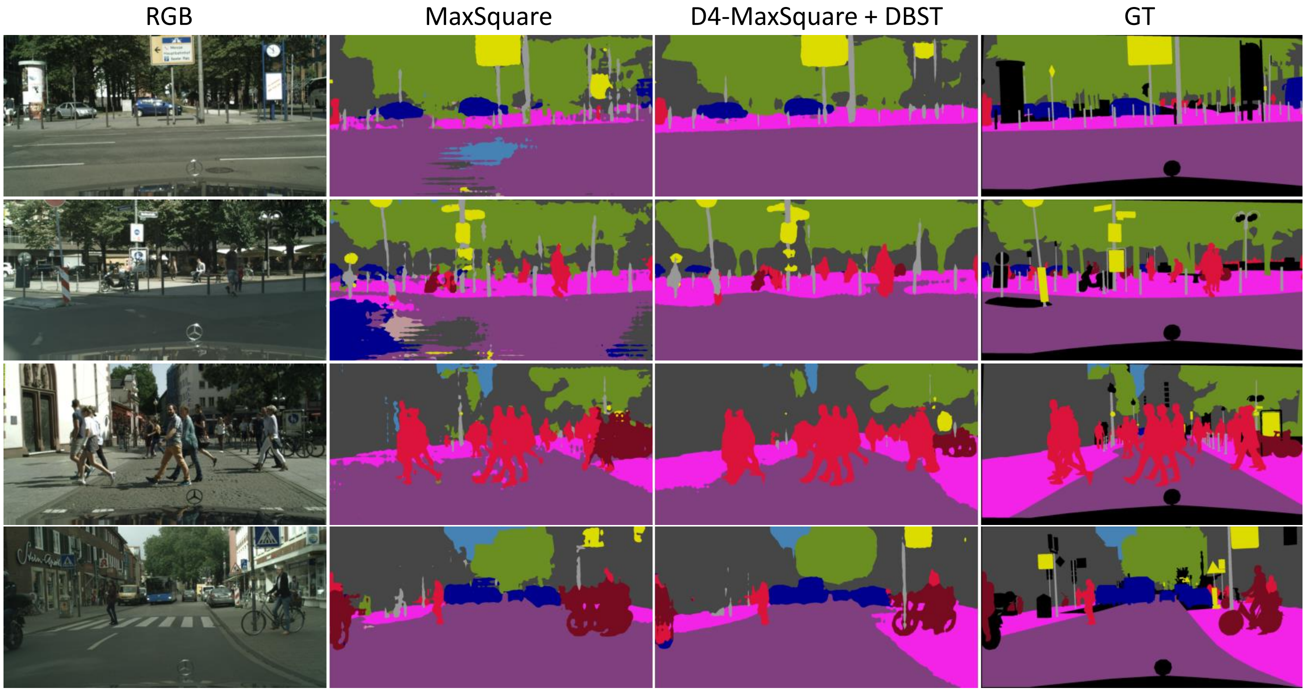


Figure 6. Qualitative results in the SYNSEQ→CS benchmark. From left to right: RGB, prediction from MaxSquare [2], prediction from D4-MaxSquare + DBST (our proposal), Ground-Truth.

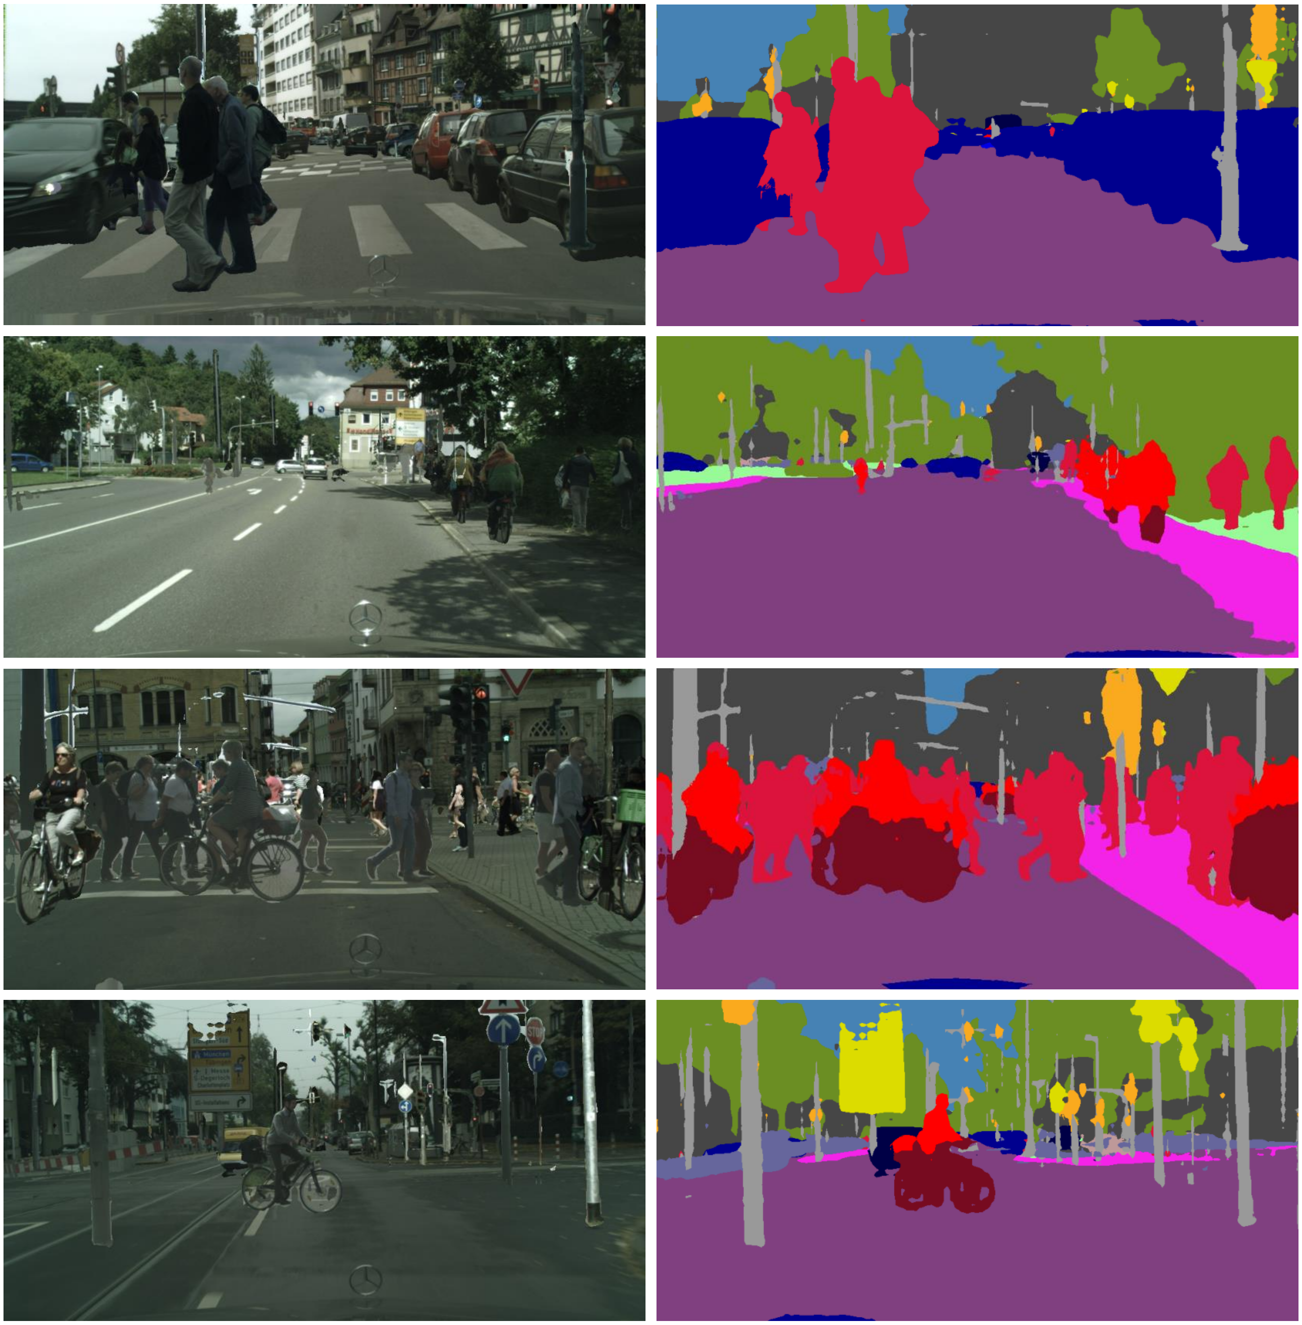

Figure 7. RGB and pseudo-labels generated for our DBST procedure using D4-LTIR in the GTA5→CS benchmark.

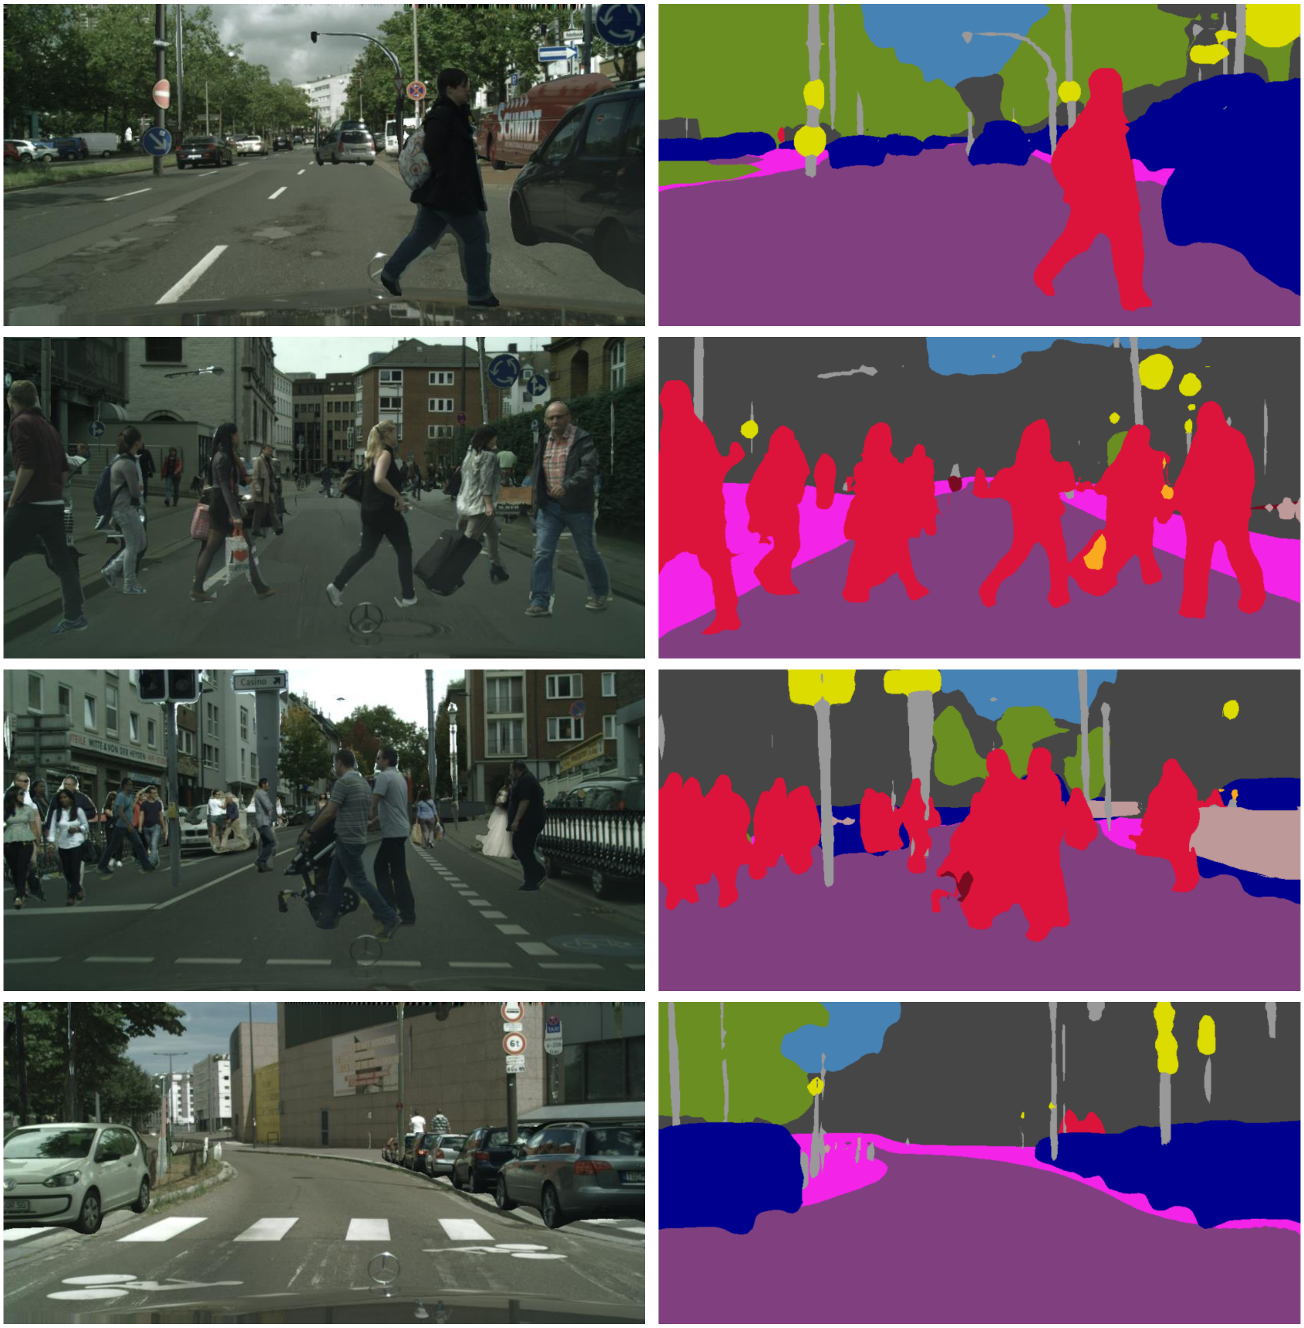

Figure 8. RGB and pseudo-labels generated for our DBST procedure using D4-MRNET in the SYNSEQ→CS benchmark.

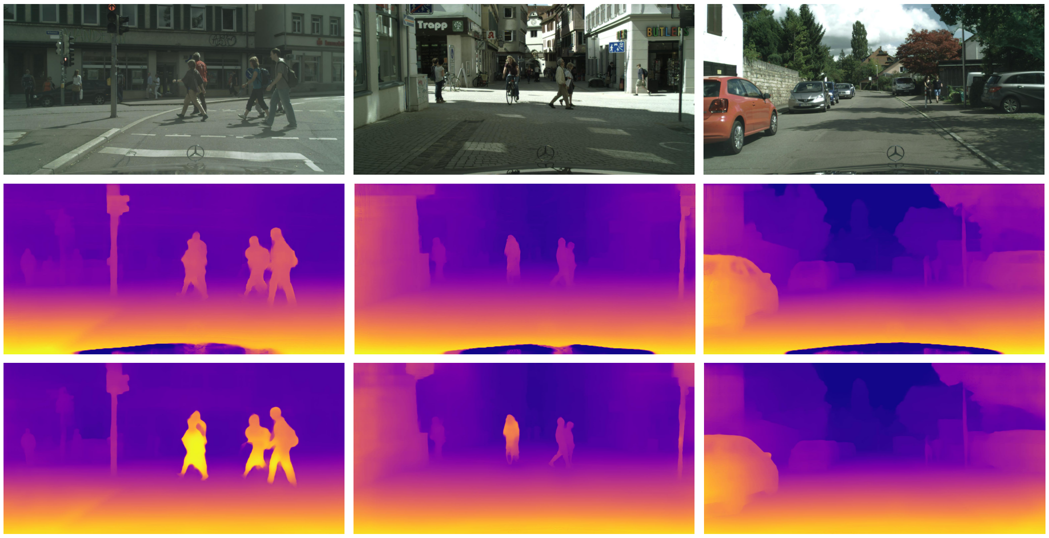


Figure 9. Depth proxy-labels for the Cityscapes dataset obtained with Monodepth2 [6]. From top to bottom: RGB, depth obtained by training Monodepth2 on Cityscapes and GTA5 sequences, depth obtained by training Monodepth2 on Cityscapes and SYNTHIA-SEQ sequences. Depth maps are shown as inverse depth maps for a better visualization.

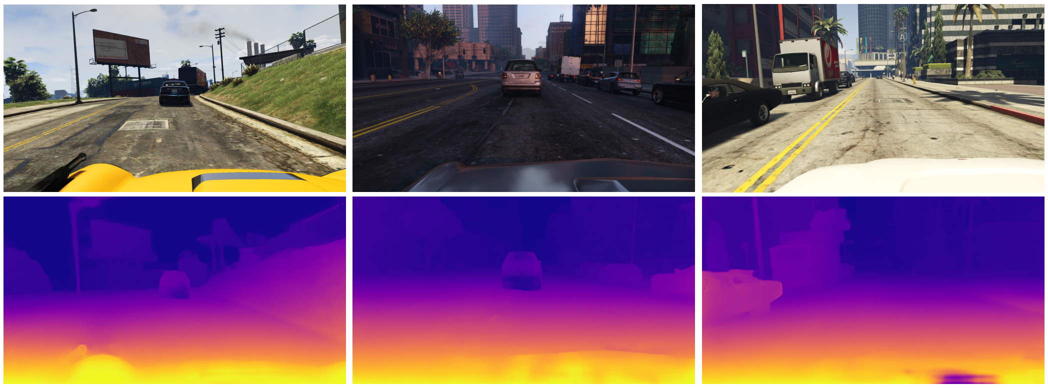

Figure 10. Depth proxy-labels for the GTA5 dataset obtained with Monodepth2 [6]. We show RGB images (first row) and corresponding depth maps (second row), shown as inverse depth maps for a better visualization.

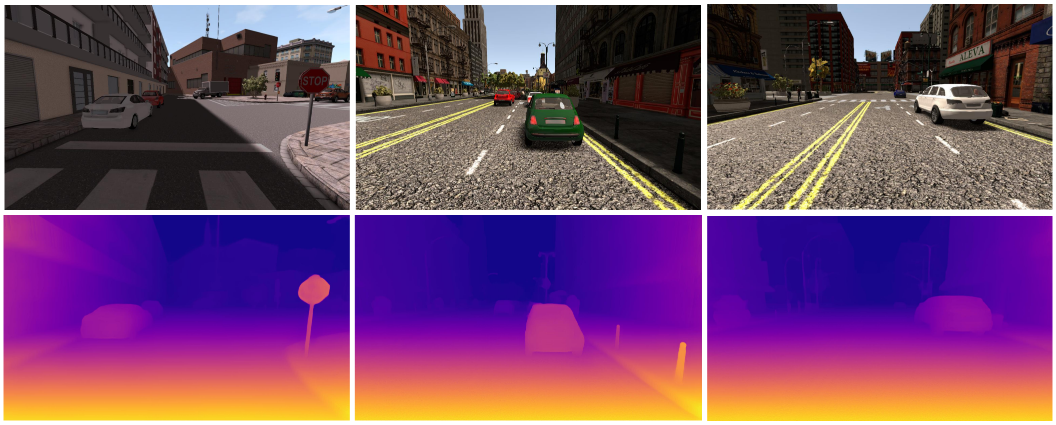


Figure 11. Depth proxy-labels for the SYNTHIA-SEQ dataset obtained with Monodepth2 [6]. We show RGB images (first row) and corresponding depth maps (second row), shown as inverse depth maps for a better visualization.
